# Supplementary material for: Probabilistic Dual Network Architecture Search on Graphs
Source: arXiv:2003.09676 source file (2020-03-21)
Supplement: Supplementary file 1 [file appendix.tex]

\appendix
\section{Activation Functions}\label{apdx:act}
\begin{table}[!h]
\caption{Different types of activation functions.}
\label{tab:act_types}
\vskip 0.15in
\begin{center}
\begin{small}
\begin{sc}
\begin{tabular}{c|l}
\toprule
Activation & Equation\\
\midrule
None & $f(x) = x$ \\
Sigmoid & $f(x) = \frac{1}{1+e^{-x}}$\\
Tanh & $ f(x) = tanh(x)$ \\
Softplus & $ f(x) = \frac{1}{\beta} \log (1+e^{\beta x})$\\
ReLU & $f(x) = Max(0,x)$ \\
LeakyReLU & $f(x) = Max(0,x) + \alpha Min(0,x)$ \\
ReLU6 & $f(x) = Min(Max(0,x),6)$ \\
ELU & $f(x) = Max(0,x) + Min(0, \alpha (e^x-1))$ \\
\bottomrule
\end{tabular}
\end{sc}
\end{small}
\end{center}
\vskip -0.1in
\end{table}

Table~\ref{tab:act_types} lists details of all types of
activation functions considered in PDNAS.

\section{Detailed Configurations}
In this section we list
the exact configurations used for all experiments.
For Adam optimiser we use different learning rates and weight decays
for different datasets but keep other parameters the same.
Specifically we set $\beta_1$ as 0.9, $\beta_2$ as 0.999, $\epsilon$ as $1e^{-8}$.
\vspace{-0.2cm}
\begin{itemize}
\item \emph{
    Citation Dataset (Semi-supervised)}:
For all 3 citation datasets in the semi-supervised setting,
we used a learning rate of 0.005 and a weight decay of $5e{-4}$
for optimising the backbone network and a learning rate of 0.002
and a weight decay of $1e{-8}$ for parameters in the NAS controller
and the routing matrix.
For each search updates we unrolled training for 30 iterations.
When searching for a 2-layer GNNs, we do not consider shortcut connections.
The number of hidden units in layers are searched
through a simple grid-search
in range of
$\{64,128,256,512\}$.
For this split we additionally
added a cosine phase in temperature annealing, as
shown in \Cref{eq:anneal}.
In practice we set $e_{cos}$ to be 100, $e_{exp}$ to be 300.

\item \emph{Citation Dataset (Fully-supervised)}:
For the fully supervised setting we randomly split the dataset
with a 6:2:2 ratio for train/validation/test datasets.
We used a learning rate of 0.001 for both optimisers.
We used a weight decay of $1e{-4}$ for the backbone network
and $1e{-8}$ for the NAS controller and routing parameters.
For each updates we unrolled training for 10 iterations.
We search over GNNs with 2 to 7 layers,
with hidden size in the range of $\{64,128,256,512\}$.
We simply used the annealing scheme mentioned in the paper (without the cosine phase).

\item \textbf{PPI Dataset:}:
PPI dataset contains 24 graphs in total.
We used 20 graphs for training,
2 graphs for validation and test separately.
This is the same as most previous approaches working on the PPI dataset.
We used a learning rate of 0.001 for both optimizers.
We do not use weight decay here.
For each updates we unrolled training for 10 iterations.
We searched over GNNs with 2 to 5 layers,
with hidden size in range $\{64,128,256,512,1024\}$.
We used the same annealing scheme as above, but choose the start epoch to be 20.

\end{itemize}
\begin{equation}\label{eq:anneal}
\tau =
\begin{cases}
    1, & \text{if } e <  e_{cos}\\
    \cos(\omega (e-e_{cos})), & e_{cos} < e < e_{exp} \\
    \mathsf{exp}^{-\frac{\alpha}{e_m} (e - e_{exp})} , & \text{otherwise}
\end{cases}
\end{equation}

\section{NAS Controller Configuration}
The NAS Controller, as discussed in the main paper,
has a graph summarisation module consisting of 2 GCN layers and 2 pooling layers,
with one Self-Attention Graph Pooling (SAGPooling) layer and a global average pooling.
The 2 GCN layers have feature transformation hidden sizes 256.
For SAGPooling we set the ratio to 0.3.
When we combine prior vector $z$ and graph embeddings $B_g$ with $W_B B_g + z$,
we initialise $W_B$ by sampling from univariate Gaussian distribution
$\mathcal{N}(0,1e^{-4})$.
The combined embedding is then processed by a MLP of size
256-256-256, and a separate linear layer then projects
the embedding to each probability vector
$P^g_{i,k}$ for sub-block $k$ in block $i$.

% \section{Search Evolution}

\begin{figure*}[!h]
    \begin{center}
		\begin{subfigure}[h]{0.25\linewidth}
        \includegraphics[width=\linewidth]{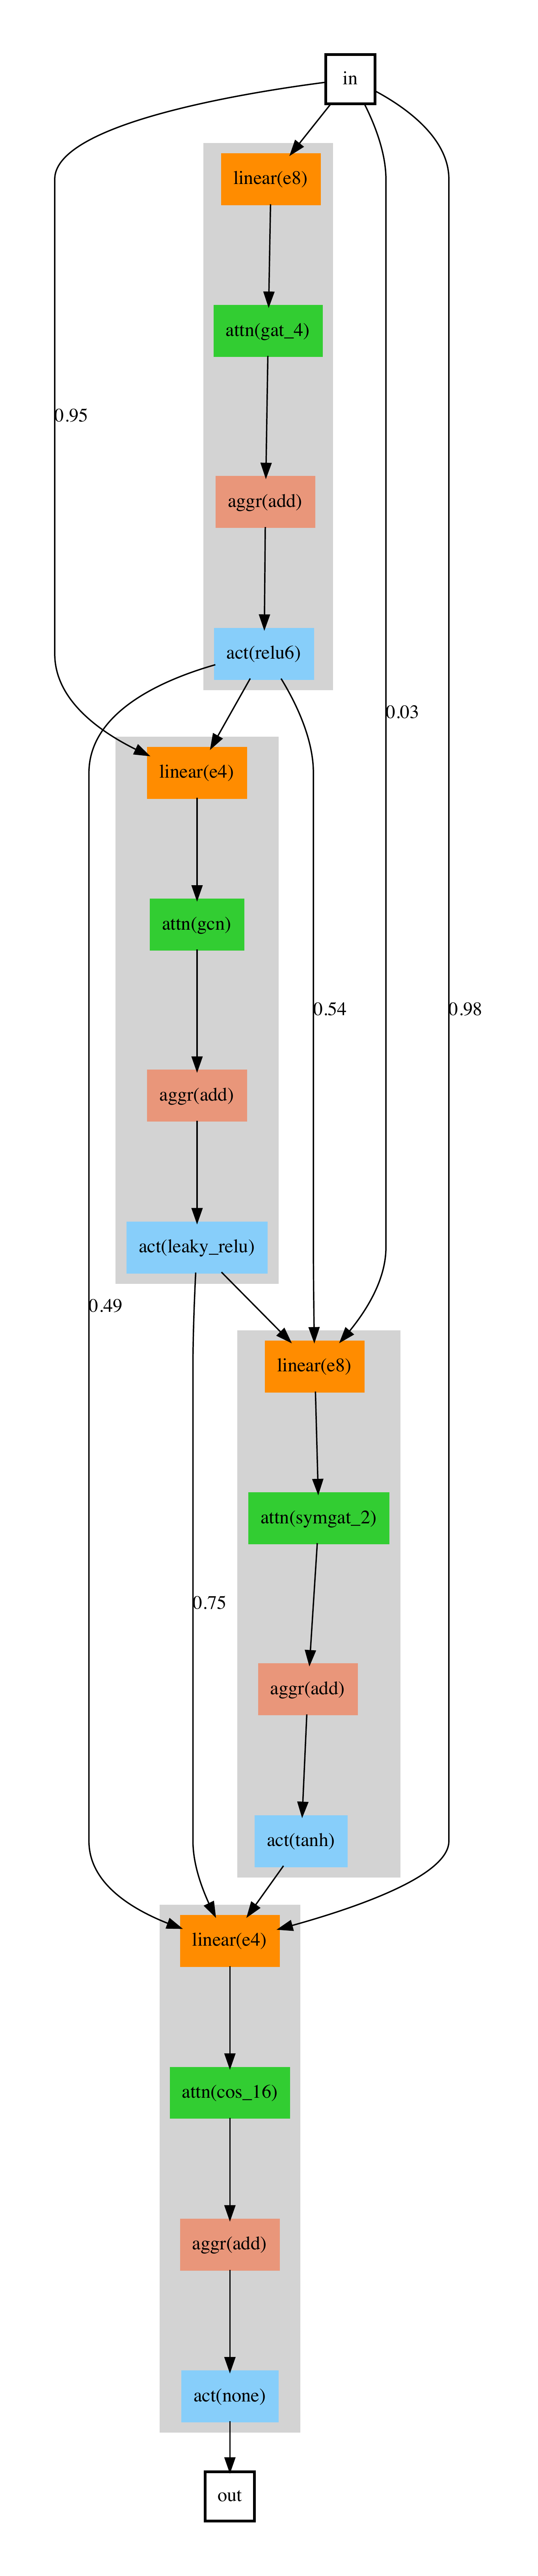}
        \caption{\label{fig:1}}
        \end{subfigure}
		\begin{subfigure}[h]{0.25\linewidth}
        \includegraphics[width=\linewidth]{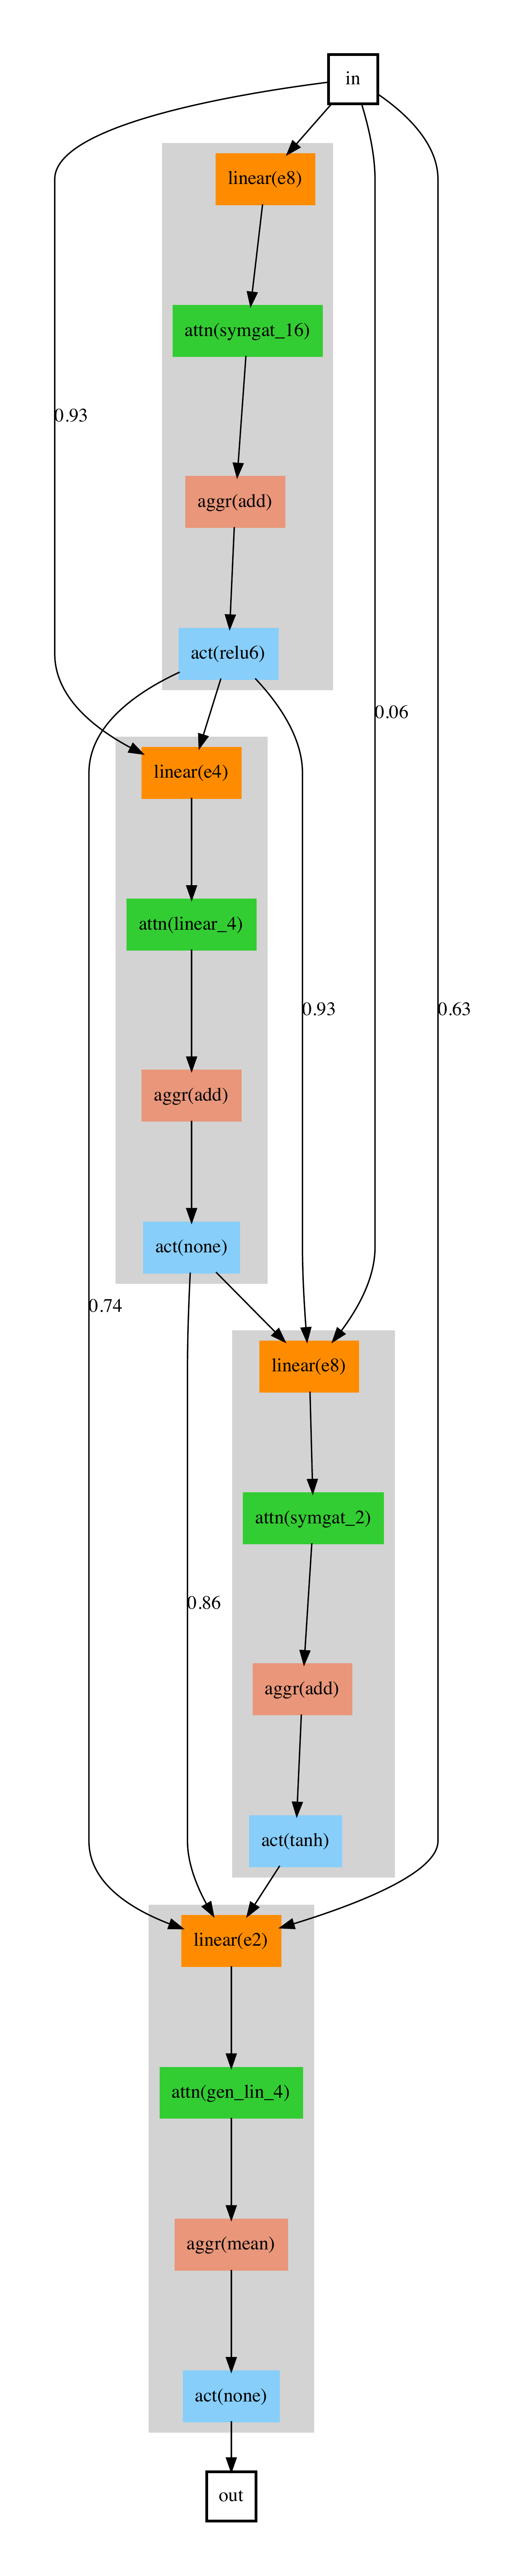}
        \caption{\label{fig:100}}
        \end{subfigure}
		% \begin{subfigure}[b]{0.2\linewidth}
		% 	\includegraphics[width=\linewidth]{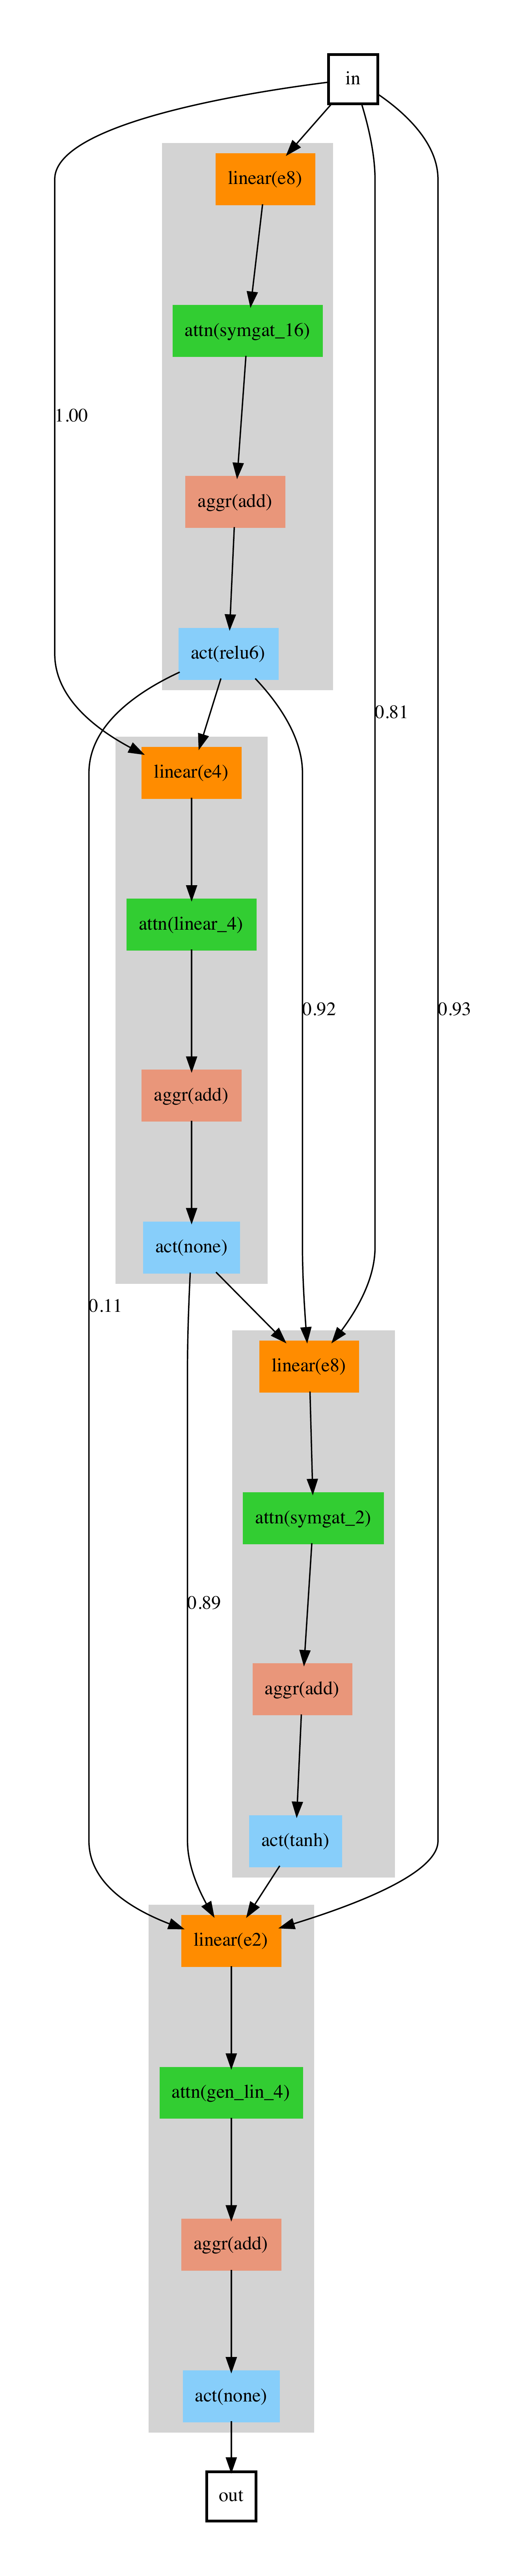}
		% 	\caption{\label{fig:200}}
		% \end{subfigure}
		\begin{subfigure}[h]{0.25\linewidth}
			\includegraphics[width=\linewidth]{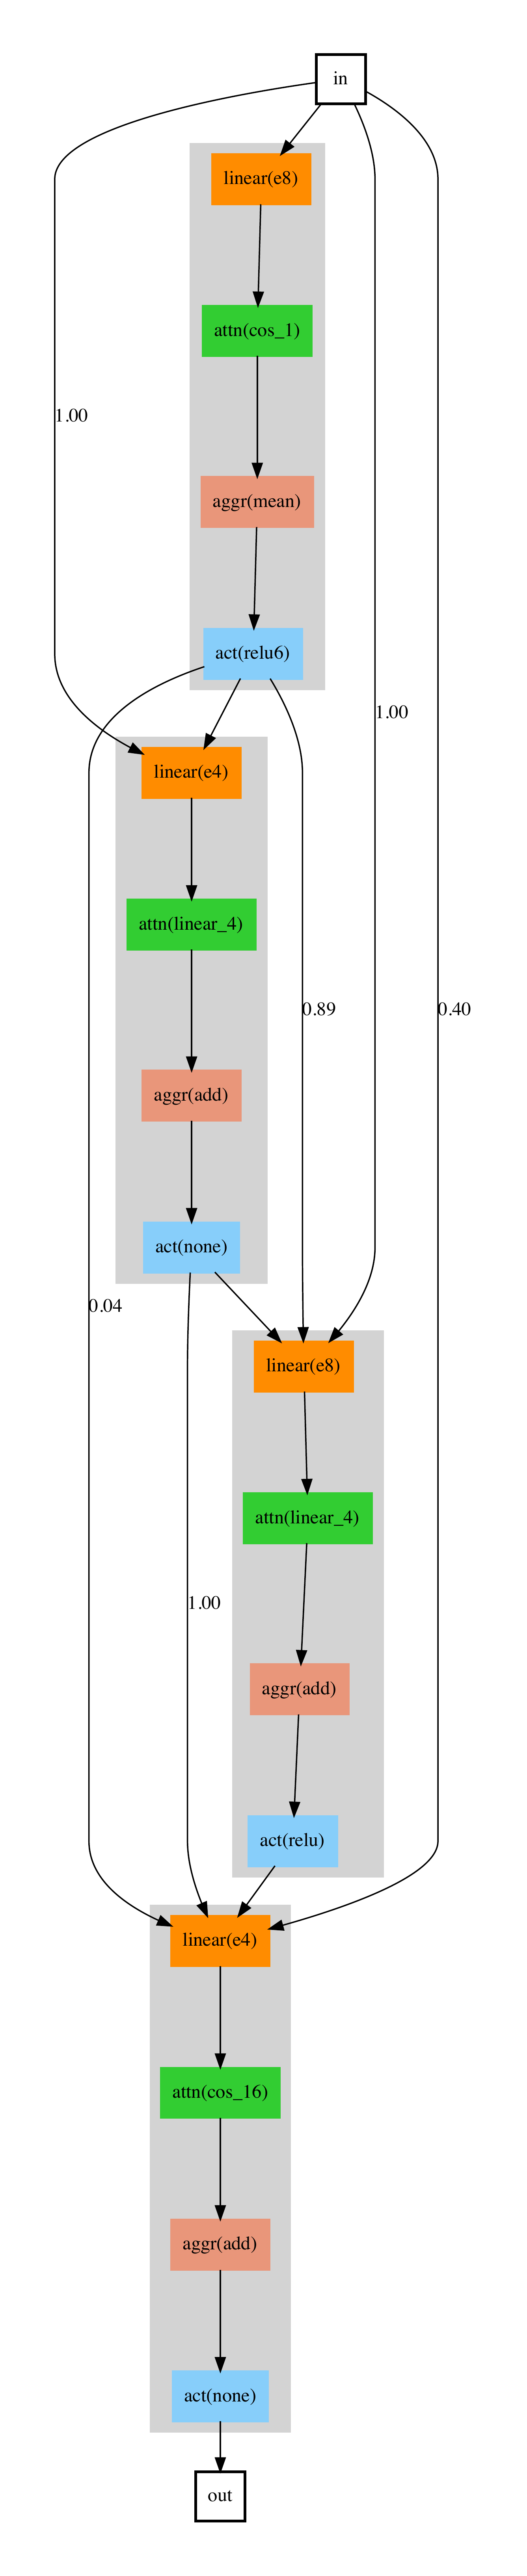}
			\caption{\label{fig:300}}
		\end{subfigure}
	\end{center}
    \caption{
        (a) Searched network architecture at epoch 1.
        (b) Searched network architecture at epoch 100.
        (c) Searched network architecture at epoch 500.
    }
	\label{fig:search}
\end{figure*}
